# Supplementary material for: Sato: Contextual Semantic Type Detection in Tables
Source: arXiv:1911.06311 source file (2020-06-03)
Supplement: Supplementary file 1 [file appendix.tex]

\begin{appendix}
\end{appendix}
